# Supplementary material for: SampleNet: Differentiable Point Cloud Sampling
Source: arXiv:1912.03663 source file (2020-04-04)
Supplement: Supplementary file 1 [file time_and_space.tex]

\begin{table}[htb!]
\begin{center}
\begin{tabular}{l c c}
\hline
Network                     &   \#Parameters    & FLOPs/        \\
                            &                   & point cloud   \\
\hline
PointNet1024                &   3.5M            & 440M          \\
PointNet32                  &   3.5M            & 14M           \\
\SPNetwo32                  &   0.22M           & 35M           \\
\SPNetwo32 with PointNet32  &   3.72M           & 49M           \\
\hline
\end{tabular}
\end{center}
\caption{{\bfseries Time and space requirements for sampled point clouds}. "M" stands for million. FLOPs is the number of multiply and accumulate operations at inference. \SPNetwo32 samples 32 points from an input of 1024 points. PointNet32 and PointNet1024 operated on the sampled and complete point clouds, respectively. When comparing the first and last rows in the table, \SPNet reduces the inference time substantially with a small increase in memory space.}
 \label{tbl:time_and_space}
\end{table}
